# Supplementary material for: SVBench: Evaluation of Video Generation Models on Social Reasoning
Source: arXiv:2512.21507 source file (2026-03-31)
Supplement: Supplementary file 1 [file X_suppl.tex]

\clearpage
\setcounter{page}{1}
\maketitlesupplementary
In this supplementary material, we detail the selection criteria for the psychological paradigms, distinguish between short-form and long-horizon tasks, and provide specific implementation configurations. 

%We also present extended experimental results, including the performance of the Wan2.2 model and evaluations of long-video generation models, followed by illustrative examples of our prompt design. 

%Finally, our datasets, generated videos, and the prompts used in our agent pipeline are available at \url{https://anonymous.4open.science/r/svbench-26AD/}

\section{Selection Criteria}
To ensure the selected psychological paradigms are suitable for evaluating social reasoning in video generation models, we established the following four criteria:

\begin{itemize}
    \item Expressibility through Observable Behavior: The experimental scenario must be conveyable purely through visible actions and interactions in a short video clip, without reliance on language, dialogue, or internal monologue.
    \item Multi-Agent Interaction: The paradigm must involve at least two agents (which can be humans, animals, or animated characters) engaged in a clear and meaningful social interaction, such as helping, hindering, imitating, or deceiving.
    \item  Well-Established and Verifiable Test Point: The paradigm must be built upon a robust, replicable finding from developmental or comparative psychology. The key test point—a specific behavior that reveals the underlying cognitive process—must be clearly defined and verifiable easliy through visual analysis of the generated video (e.g., an agent's gaze direction, choice of object, or manner of action).
    \item Configurable Cognitive Demand: The paradigm should allow for the adjustment of its social or causal complexity. This enables the creation of multiple variants to probe the model's sensitivity, for example, by varying the number of social cues, the salience of the goal, or the plausibility of an outcome. 
\end{itemize}
Based on these criteria, we searched through a large amount of classic psychology content and ultimately selected 30 seed experiments.

\section{Long and short division}
A core premise of our benchmark is that evaluating social reasoning requires moving beyond static scene descriptions to dynamic scenarios defined by precondition actions and logical sequences. This demands that a model not only understands a complex, multi-part instruction but can also infer plausible character reactions based on the social logic embedded within those instructions.

To systematically assess this capability across varying levels of difficulty, we categorize our tasks into two types:

\begin{itemize}
    \item Short-form Tasks: These tasks, which form the basis of the 15 evaluations in the main paper, are designed to test fundamental social reasoning concepts. They typically involve a concise sequence of actions that can be adequately depicted within a short video clip (aligned with the 5-12 second range common among current SOTA models). The challenge here is for the model to correctly interpret the immediate social cue and generate the corresponding, logically sound interaction.
    \item  Long-horizon Tasks: Many classic tests of advanced social reasoning (e.g., tests of false belief, complex deception) require a longer narrative structure to establish necessary preconditions. A single short clip is insufficient to set up the multiple steps of actions and mental state changes that lead to the critical test point. Generating such long-horizon scenarios is currently a significant challenge for models, both due to technical limitations in maintaining coherence over time and the high computational cost.
\end{itemize}

\section{Implementation Details}
In our short-video experiments, all generated videos were constrained to a length of 5–10 seconds. Specifically, the four closed-source models were configured to generate 8-second videos, while open-source models uniformly produced 5-second videos. For the long-video experiment, a fixed duration of 30 seconds was used for all generations. To ensure consistent output quality, all open-source models were evaluated using their 14B parameter versions at 720p resolution. The testing of open-source models was conducted across a total of 32 H800 GPUs to accommodate the computational demands of the experiment.

\section{Long Video Results}
Considering the substantial computational time required for long video generation, we evaluated a subset of three specialized models—Self-Forcing \cite{huang2025self}, LongLive \cite{yang2025longlive}, and Skyreels-v2 \cite{chen2025skyreels}—under the long-video setting. In contrast to the short-video experiments, each seed scenario here corresponds to a single scene articulated across three difficulty gradients. The complete results are summarized in Table~\ref{tab:experiment_results_long}. 

Overall, performance on long-video generation remains considerably lower than that observed in short videos, with the best model achieving only 22.7\% accuracy. This suggests that current models still struggle to maintain coherent character interactions and social reasoning over extended sequences. Among the evaluated models, LongLive demonstrates a relative advantage in several tasks such as Level 1 Visual Perspective Taking, whereas Self-Forcing shows competitive results in Cooperative Deception Detection. Skyreels-v2 exhibits a mixed profile, performing strongly in certain perspective-taking tasks but lagging in most social reasoning scenarios. These results underscore the significant challenge that long-horizon social reasoning continues to pose for contemporary video generation systems.

\begin{table*}[t]
\centering
\scriptsize
\caption{\textbf{Experimental Results for long video generation models.} We report the performance (\%) of three models on tasks grouped by social reasoning dimensions.}
\label{tab:experiment_results_long}
% Reduce the space between columns to help the table fit
\setlength{\tabcolsep}{4pt}
\begin{tabular}{l@{\hskip 1em}l@{\hskip 1em}ccc}
\toprule
\multirow{2}{*}{\textbf{Task Dimension}} & \multirow{2}{*}{\textbf{Sub-Task}} & \multicolumn{3}{c}{\textbf{Model Performance (\%)}} \\
\cmidrule(lr){3-5}
 & & 
 \rotatebox{45}{\textbf{LongLive}} & 
 \rotatebox{45}{\textbf{Self-Forcing}} & 
 \rotatebox{45}{\textbf{Skyreels-v2}} \\
\midrule    
\multirow{5}{*}{Mental State Reasoning} 
 & Sally-Anne Test  & 33.3 & 40.0 &  6.7  \\
 & Smarties Task & 6.7 & 20.0 &    20.0 \\
 & Level 2 Visual Perspective Taking & 20.0  & 40.0 & 26.7    \\
 & Knowledge Access & 33.3 & 6.7 &   6.7  \\
 & Intentional vs Accidental Actions & 20.0 & 6.7 & 6.7    \\
\midrule
\multirow{3}{*}{Goal Directed Action}
 & Kohler Stick &40  & 26.7 &  33.3     \\
 & Gergely's Head-Touch & 20.0 & 6.7 & 20.0    \\ 
 & Failed Attempts & 6.7 & 6.7 & 6.7    \\
\midrule      
\multirow{1}{*}{Joint Attention and Perspective}
 & Level 1 Visual Perspective Taking & 46.7 & 13.3 & 80.0    \\  
\midrule 
\multirow{2}{*}{Social Coordination}
 & Collaborative Transport  & 20.0 & 20.0 & 20.0  \\  
 & Collision Avoidance Pedestrian Flow  &13.3  &6.7  & 6.7   \\
\midrule 
\multirow{4}{*}{Multi-Agent Social Strategy} 
 & Competitive Resource Allocation & 6.7 & 6.7 &   6.7  \\
 & Cooperative Deception Detection & 33.3 & 60 & 33.3    \\
 & Norm Violation Response & 20.0 & 6.7 & 6.7   \\
 & Multi-Party Collaborative Problem Solving & 26.7 & 13.3 & 46.7     \\
\midrule
Overall 
 & - & 22.7 & 17.8 & 20.4    \\
\bottomrule
\end{tabular}
\end{table*}

\section{Prompt Design Examples}
Our benchmark employs a structured prompt design in which each social reasoning experiment is defined by several key components. As illustrated in Table~\ref{tab:example_prompts}, every experiment specifies: (1) multiple prompt variants across difficulty levels, each describing observable behaviors while excluding internal mental states; (2) ground truth annotations derived from established psychological findings; and (3) a standardized evaluation question designed to elicit a behaviorally verifiable response.

For every psychological paradigm, prompts are constructed from a minimal, structured description. Difficulty levels are systematically manipulated by varying the explicitness of social cues: Easy prompts incorporate clear, detailed, indicators that strongly support the target inference; Medium prompts introduce subtler cues that remain informative yet require greater integration; and Hard prompts are phrased in sparse, context-only language, demanding inference from minimal behavioral information.

The implementation of difficulty progression varies by paradigm. In Empathic Concern, difficulty increases as explicit comforting cues are progressively removed—from direct physical engagement like kneeling with open arms (Easy), to a clear attentional orientation like turning to look (Medium), and finally to mere spatial proximity without clear interactive intent (Hard). In Gaze Following, difficulty escalates as supplementary cues are eliminated: beginning with combined gaze and an explicit pointing gesture (Easy), proceeding to gaze with an implied attentional shift in the observer (Medium), and culminating in gaze direction alone without any additional indicators (Hard).

\begin{table*}[h]
\centering
\caption{Examples for Empathic Concern and Gaze Following}
\label{tab:example_prompts}
\small
\begin{tabular}{p{1.1cm} p{1.8cm} p{4cm} p{3.2cm} p{3.2cm}}
\toprule
\textbf{Exp.} & \textbf{Difficulty} & \textbf{Prompt} & \textbf{Ground Truth} & \textbf{Question} \\
\midrule

\multirow{3}{*}{\rotatebox[origin=c]{90}{\parbox{1.8cm}{\centering Empathic Concern}}}
& Easy & A little girl is crying over a dropped ice cream. A woman kneels down in front of her and opens her arms. & The woman will hug or verbally comfort the girl. & What will the woman do next? \\
\cmidrule(lr){2-5}
& Medium & A little girl is crying next to her dropped ice cream. A woman nearby turns to look directly at the crying girl. & The woman will approach and comfort the girl. & What is the woman likely to do? \\
\cmidrule(lr){2-5}
& Hard & A girl is crying on a park bench. A dropped ice cream cone is on the ground nearby. A woman is sitting on the other end of the bench. & The woman will notice the crying girl and offer comfort. & Describe the most likely interaction between the woman and the girl. \\
\midrule

\multirow{3}{*}{\rotatebox[origin=c]{90}{\parbox{1.8cm}{\centering Gaze Following}}}
& Easy & A woman looks toward a red toy on the floor and then briefly points at it. A boy beside her is looking at her. & Boy will look at the red toy on the floor. & Does the boy look at the red toy on the floor? \\
\cmidrule(lr){2-5}
& Medium & A woman directs her gaze toward a red toy on the floor. The boy beside her, who is looking at her, seems to notice her shift in attention. & Boy will look at the red toy on the floor. & Does the boy look at the red toy on the floor? \\
\cmidrule(lr){2-5}
& Hard & A woman directs her gaze toward a red toy on the floor. A boy is beside her, looking at the woman. & Boy will look at the red toy on the floor. & Does the boy look at the red toy on the floor? \\

\bottomrule
\end{tabular}
\end{table*}

\begin{figure*}[t]
    \centering
    \includegraphics[width=\linewidth]{sec/fig/badcase.pdf}
    \caption{\textbf{Failure example of LongLive on the \emph{Sally-Anne} false-belief task.} The prompt requires the woman to leave the room while the girl hides the toy mouse in the red bag, but in the generated video she never exits and the toy remains in the blue shoe box, revealing failures in instruction following and social reasoning.}
    \label{fig:longlive_failure}
\end{figure*}

\section{Qualitative Case Study of a Failure Example}
To complement the quantitative results in Table~\ref{tab:experiment_results_long}, we provide a qualitative case study of a single failure example from a long-video generation model. The example is based on the \emph{Sally-Anne} false-belief paradigm and is instantiated using the LongLive model~\cite{yang2025longlive}.

In this scenario, the prompt describes a woman standing by a table with a blue shoe box containing a toy mouse and a red bag nearby. The woman is instructed to place the toy mouse into the blue shoe box and then leave the room. While she is away, a girl secretly takes the toy mouse from the blue shoe box and hides it in the red bag. Finally, the woman returns, intending to retrieve the toy. This setup is designed to instantiate a classic false-belief structure: the critical test point is whether the woman’s subsequent action reflects her outdated belief that the toy is still in the blue shoe box.

However, the generated video reveals two notable failures. First, the model shows \textbf{weak instruction-following ability}: although the prompt explicitly requires the woman to leave the room to establish her ignorance of the relocation event, she never actually exits the scene in the generated sequence. Second, the model exhibits \textbf{limited social reasoning ability}. After the girl moves the toy, the woman does not engage in any belief-consistent search behavior—she neither checks the red bag nor displays any visually interpretable reaction to the toy’s absence. Instead, the toy continues to appear in the blue shoe box, indicating that the model fails to maintain a coherent world state and to generate behavior consistent with the underlying false-belief logic.

This single case illustrates how current long-video models can produce locally plausible frames while still violating the global social-cognitive structure prescribed by the prompt. It highlights the importance of benchmarks that evaluate not only visual fidelity but also the consistency of generated behavior with the underlying social reasoning structure specified by the task.
